# Supplementary material for: Ultramassive black holes formed by triple quasar mergers at $z\sim 2$
Source: arXiv:2209.01249 source file (2022-09-07)
Supplement: Supplementary file 1 [file Sec6_Appendix.tex]

% \begin{figure}
% \centering
%   \includegraphics[width=1.0\columnwidth]{plots/QLF_z23.png}
%   \caption{Bolometric luminosity of BHs at $z=2.3$. Observation data compiled by Shen2020}
%   \label{fig:QLF}
% \end{figure}
